# Supplementary material for: On the Convergence of Reinforcement Learning in Nonlinear Continuous State Space Problems
Source: arXiv:2011.10829 source file (2021-07-28)
Supplement: Supplementary file 1 [file Appendix.tex]

\clearpage

\section*{APPENDIX}

\subsection{Proof of Lemma \ref{L1}}
\label{sec:proofL1}

\begin{proof}
We proceed by induction. The first general instance of the recursion occurs at $t=3$.
It can be shown that: 
 \begin{align}
 &\delta x_3 = \underbrace{(\bar{A}_2\bar{A}_1(\epsilon w_0) + \bar{A}_2 (\epsilon w_1) + \epsilon w_2)}_{\delta x_3^l} + \nonumber\\
 &\underbrace{\{\bar{A}_2 \bar{S}_1(\epsilon w_0) + \bar{S}_2(\bar{A}_1(\epsilon w_0) + \bar{S}_2(\bar{A}_1(\epsilon w_0) + \epsilon w_1 + \bar{S}_1(\epsilon w_0))\}}_{\bar{\bar{S}}_3}. 
 \end{align}
 Noting that $\bar{S}_1(.)$ and $\bar{S}_2(.)$ are second and higher order terms, it follows that $\bar{\bar{S}}_3$ is $O(\epsilon^2)$. \\
 Suppose now that $\delta x_t = \delta x_t^l + \bar{\bar{S}}_t$ where $\bar{\bar{S}}_t$ is $O(\epsilon^2)$. Then:
 \begin{align}
 \delta x_{t+1} = \bar{A}_{t+1}(\delta x_t^l + \bar{\bar{S_t}}) + \epsilon w_t + \bar{S}_{t+1}(\delta x_t), \nonumber\\
 = \underbrace{(\bar{A}_{t+1} \delta x_t^l + \epsilon w_t)}_{\delta x_{t+1}^l} +\underbrace{\{\bar{A}_{t+1}\bar{\bar{S}}_t + \bar{S}_{t+1}(\delta x_t)\}}_{\bar{\bar{S}}_{t+1}}.
 \end{align}
 Noting that $\bar{S}_{t+1}$ is $O(\epsilon^2)$ and that $\bar{\bar{S}}_{t+1}$ is $O(\epsilon^2)$ by assumption, the result follows. 
\end{proof}

\subsection{Proof of Proposition \ref{prop1}}
\label{sec:proofP1}

\begin{proof}
From \eqref{eq.9b}, we get,
\begin{align} 
\tilde{J}^{\pi} = \mathbb{E}[J^{\pi}] =  \mathbb{E}[ \bar{J}^{\pi} + \delta J_1^{\pi} + \delta J_2^{\pi}], \nonumber\\
= \bar{J}^{\pi} + \mathbb{E}[\delta J_2^{\pi}]  = \bar{J}^{\pi} + O(\epsilon^2), \label{eq.10}
%= \bar{J}_0^{\pi} + \underbrace{ \mathbb{E}[\delta J_2^{\pi}]}_{\delta \tilde{J}_2^{\pi}} = \bar{J}^{\pi}_0 + O(\epsilon^2). \label{eq.10}
\end{align}
The first equality in the last line of the equations before follows from the fact that $\mathbb{E}[\delta x_t^l] = 0$, since its the linear part of the state perturbation driven by white noise and by definition $\delta x_1^l = 0$.The second equality follows form the fact that $\delta J_2^{\pi}$ is an $O(\epsilon^2)$ function.  Now,
\begin{align}
\text{Var}(J^{\pi}) = \mathbb{E}[ J^{\pi} - \tilde{J}^{\pi}]^2 \nonumber\\
= \mathbb{E}[ \bar{J}_0^{\pi} + \delta J_1^{\pi} + \delta J_2^{\pi} - \bar{J}_0^{\pi} - \delta \tilde{J}_2^{\pi}]^2 \nonumber\\
= \text{Var}(\delta J_1^{\pi}) + \text{Var}(\delta J_2^{\pi})  + 2 \mathbb{E}[\delta J_1^{\pi} \delta J_2^{\pi}].
\end{align}
Since $\delta J_2^{\pi}$ is $O(\epsilon^2)$, $\text{Var}(\delta J_2^{\pi})$ is an $O(\epsilon^4)$ function. It can be shown that $\mathbb{E}[\delta J_1^{\pi} \delta J_2^{\pi}]$ is $O(\epsilon^4)$ as well (proof is given \citep{d2cTR}). Finally $\text{Var}(\delta J_1^{\pi})$ is an $O(\epsilon^2)$ function because $\delta x^l$ is an $O(\epsilon)$ function. Combining these, we will get the desired result. 
\end{proof} 

\subsection{Proof of Proposition \ref{prop2}}
\label{sec:proofP2}

\begin{proof}
We have 
\begin{align*}
\tilde{J}^{\pi^*} - \tilde{J}^{\pi^o}  &= \tilde{J}^{\pi^*} -  \bar{J}^{\pi^*} + \bar{J}^{\pi^*} -  \tilde{J}^{\pi^o}  \\
&\leq \tilde{J}^{\pi^*} -  \bar{J}^{\pi^*} + \bar{J}^{\pi^{o}} -  \tilde{J}^{\pi^o}
\end{align*}
The  inequality above is due the fact that $\bar{J}^{\pi^*} \leq \bar{J}^{\pi^{o}}$, by definition of $\pi^{*}$. Now, using Proposition \ref{prop1}, we have that $|\tilde{J}^{\pi^*} - \bar{J}^{\pi^*}| = O(\epsilon^2)$, and $|\tilde{J}^{\pi^o} -  \bar{J}^{\pi^o}| = O(\epsilon^2)$. Also, by definition, we have $\tilde{J}^{\pi^o} \leq   \tilde{J}^{\pi^*}$. Then, from the above inequality, we get 
\begin{align*}
| \tilde{J}^{\pi^*} - \tilde{J}^{\pi^o} | \leq |\tilde{J}^{\pi^*} -  \bar{J}^{\pi^*} | + | \bar{J}^{\pi^{o}} -  \tilde{J}^{\pi^o} | = O(\epsilon^{2})
\end{align*}
A similar argument holds for the   variance as well. \\[10pt]
\end{proof}

\subsection{Lemma 2}
\label{sec:proofL2}

\begin{lemma} 
\label{L2}
Let $\delta J_1^{\pi}$, $\delta J_2^{\pi}$ be as defined in \eqref{eq.9b}. Then, $\mathbb{E} [\delta J_1 \delta J_2]$ is an $O(\epsilon^4)$ function.
\end{lemma}

\begin{proof}
In the following, we suppress the explicit dependence on $\pi$ for $\delta J_1^{\pi}$ and $\delta J_2^{\pi}$ for notational convenience.
Recall that $\delta J_1 = \sum_{t=0}^T c_t^x \delta x_t^l$, and $\delta J_2 = \sum_{t=0}^T \bar{H}_t(\delta x_t) + c_t^x \bar{\bar{S}}_t$.  For notational convenience, let us consider the scalar case, the vector case follows readily at the expense of more elaborate notation. Let us first consider $\bar{\bar{S}}_2$. We have that $\bar{\bar{S}}_2 = \bar{A}_2\bar{S}_1(\epsilon w_0) + \bar{S}_2(\bar{A}_1(\epsilon w_0) + \epsilon w_1+ \bar{S}_1(\epsilon w_0))$. Then, it follows that:
\begin{align}
\bar{\bar{S}}_2 = \bar{A}_2 \bar{S}_1^{(2)}(\epsilon w_0)^2 + \bar{S}_2^{(2)}(\bar{A}_1 \epsilon w_0 + \epsilon w_1)^2 + O(\epsilon^3),
\end{align}
where $\bar{S}_t^{(2)}$ represents the coefficient of the second order term in the expansion of $\bar{S}_t$. A similar observation holds for $H_2(\delta x_2)$ in that:
\begin{align}
\bar{H}_2(\delta x_2) = \bar{H}_2^{(2)}(\bar{A}_1(\epsilon w_0) + \epsilon w_1)^2 + O(\epsilon^3),
\end{align}
where $\bar{H}_t^{(2)}$ is the coefficient of the second order term in the expansion of $\bar{H}_t$. Note that $\epsilon w_0 = \delta x_1^l$ and $\bar{A}_1(\epsilon w_0) + \epsilon w_1= \delta x_2^l$. Therefore, it follows that we may write:
\begin{align}
\bar{H}_t(\delta x_t) + C_t^x \bar{\bar{S}}_t = \sum_{\tau = 0}^{t-1} q_{t,\tau}(\delta x_{\tau}^l)^2 + O(\epsilon^3),
\end{align}
for suitably defined coefficients $q_{t,\tau}$. 
Therefore, it follows that 
\begin{align}
\delta J_2 = \sum_{t=1}^T \bar{H}_t(\delta x_t) + C_t^x \bar{\bar{S}}_t\nonumber\\
= \sum_{\tau = 0}^T \bar{q}_{T,\tau}(\delta x_{\tau}^l)^2+ O(\epsilon^3),
\end{align}
for suitably defined $\bar{q}_{T,\tau}$. Therefore:
\begin{align}
\delta J_1 \delta J_2 = \sum_{t,\tau} C_{\tau}^x(\delta x_{\tau}^l)\bar{q}_{T,t}(\delta x_t^l)^2 + O(\epsilon^4).
\end{align}
Taking expectations on both sides:
\begin{align}
E[\delta J_1 \delta J_2] = \sum_{t,\tau} C_{\tau}^x \bar{q}_{T,t} E[\delta x_{\tau}^l (\delta x_t^l)^2] + O(\epsilon^4).
\end{align}
Break $\delta x_t^l = (\delta x_t^l - \delta x_{\tau}^l) + \delta x_{\tau}^l$, assuming $\tau < t$. Then, it follows that:
\begin{align}
E[\delta x_{\tau}^l (\delta x_t^l)^2] = E[\delta x_{\tau}^l (\delta x_t^l - \delta x_{\tau}^l)^2] + E[(\delta x_{\tau}^l)^3]  \nonumber\\
+ 2 E[(\delta x_t^l - \delta x_{\tau}^l)(\delta x_{\tau}^l)^2]\nonumber\\
= E[(\delta x_{\tau}^l)^3],
\end{align}
where the first and last terms in the first equality drop out due to the independence of the increment $(\delta x_t^l - \delta x_{\tau}^l)$ from $\delta x_{\tau}^l$, and the fact that $E[\delta x_t^l - \delta x_{\tau}^l] = 0$ and $E[\delta x_{\tau}^l] = 0$. Since $\delta x_{\tau}^l$ is the state of the linear system $\delta x_{t+1}= \bar{A}_t \delta x_t^l + \epsilon w_t$, it may again be shown that:
\begin{align}
E[\delta x_{\tau}^l]^3 = \sum_{s_1,s_2,s_3} \Phi_{\tau, s_1}\Phi_{\tau,s_2}\Phi_{\tau,s_3} E[w_{s_1}w_{s_2}w_{s_3}],
\end{align}
where $\Phi_{t,\tau}$ represents the state transitions operator between times $\tau$ and $t$, and follows from  the closed loop dynamics. Now, due to the independence of the noise terms $w_t$, it follows that $E[w_{s_1}w_{s_2}w_{s_3}] = 0$ regardless of $s_1,s_2,s_3$.\\
 An analogous argument as above can be repeated for the case when $\tau > t$. Therefore, it follows that $E[\delta J_1 \delta J_2] = O(\epsilon^4)$.
\end{proof}
